# Supplementary material for: SceneLoom: Communicating Data with Scene Context
Source: arXiv:2507.16466 source file (2025-07-28)
Supplement: Supplementary file 1 [file 8-appendix.tex]

\newpage
\section*{Supplementary Materials}

\section{Implementation Details}
This section presents the prompt examples described in Sec.4, with their corresponding output examples.

\subsection{Data Preparation}
This section provides examples of prompts and output results mentioned in Sec.4.2, including feature extraction from narrative intent and data table and data visualization generation. 
%% feature extraction
\begin{coloredquotation}
    \textbf{Prompt template for feature extraction:}\\
You are an expert in data analysis and data-driven storytelling. You need to extract data-related information, entity objects, and actions to guide animations based on the narrative intent \{\textit{narrative intent}\} and the corresponding data table \{\textit{data}\}. Some explanations are as follows:

\# Data-related information

- Data fact: Extract all key data points and insights directly from the narration, avoiding redundancy. Insights should be derived primarily from the narration, with data used as supporting evidence rather than being the sole source of information.

- Metadata: Provide structured metadata to support visualization and data transformation, including relevant data columns and data transformation methods.

\# Entity objects: Identify real-world objects or concepts that have explicit semantic meaning and could be represented visually.

\# Actions

- Enter: Describe how elements should appear in the visualization, including the sequence or transition style.

- Emphasize: Highlight key information using animation techniques, specifying what should be emphasized and how.

The output should be in the following JSON format:
\begin{lstlisting}[language=TypeScript, label={lst:visualization-class}]
{
  "dataRelatedInformation": {
    "dataFact": [],
    "metadata": {
      "dataColumns": [],
      "dataTransformation": []
    }
  },
  "entityObjects": [],
  "actions": [
    {"enter": ""},
    {"emphasize": ""},
  ]
}
\end{lstlisting}
\end{coloredquotation}

An example of extracted features:
\begin{lstlisting}[language=json, label={lst:visualization-class}]
{
  "dataRelatedInformation": {
    "dataFact": [
      "46% of Americans prefer artificial trees, while 26% prefer real ones.",
      "Over recent decades, there has been a steady increase in the use of artificial trees."
    ],
    "metadata": {
      "dataColumns": ["Response", "Share of Respondents (%)"],
      "dataTransformation": [
        "Sort 'Response' column in descending order based on 'Share of Respondents (%)'."
      ]
    }
  },
  "entityObjects": ["Artificial Christmas tree", "Real Christmas tree", "Survey respondents"],
  "actions": [
    {
      "enter": "Introduce the growing preference for artificial trees over real trees using a transition animation."
    },
    {
      "emphasize": "Highlight the 46% artificial tree preference in the US by making the corresponding bar pulse or grow slightly."
    }
  ]
}
\end{lstlisting}

%% data visualization generation
Data visualizations are generated using d3.js. We have designed multiple d3.js-based visualization interfaces to create consistent yet flexible visualization variants (e.g., horizontal histogram, vertical histogram). Thus, the task here is to generate the required interface parameters. Furthermore, we leverage data-related information from prior feature extraction to produce more related visualization alternatives.
\begin{coloredquotation}
    \textbf{Prompt template for data visualization generation:}\\
You are an expert in data visualization and data analysis. 
You need to generate as many appropriate visualization charts as possible based on the data information \{\textit{dataRelatedInformation}\} and data table \{\textit{data}\}.

The output should be in the following JSON format:
\begin{lstlisting}[language=TypeScript, label={lst:visualization-class}]
{
  //"bar-0", "line-0", "line-1"
  "chartId": "", 
  "type": "",
  //Categorical data, only list the column name
  "categoryKey": [], 
  //Numerical data, only list the column name(s)
  "valueKeys": [], 
  //Title of the chart
  "title": ""
}
\end{lstlisting}
\end{coloredquotation}

An example of visualization generation parameters:
\begin{lstlisting}[language=json, label={lst:visualization-class}]
[
    {
        "chartId": "bar-0",
        "type": "vertical",
        "categoryKey": ["Response"],
        "valueKeys": ["Share of Respondents (%)"],
        "title": "Distribution of Respondents",
    },
    {
        "chartId": "bar-1",
        "type": "horizontal",
        "categoryKey": ["Response"],
        "valueKeys": ["Share of Respondents (%)"],
        "title": "Distribution of Respondents",
    },
    {
        "chartId": "line-0",
        "type": "basic",
        "categoryKey": ["Response"],
        "valueKeys": ["Share of Respondents (%)"],
        "title": "Trends in Tree Preferences",
    },
    {
        "chartId": "line-1",
        "type": "with-dot",
        "categoryKey": ["Response"],
        "valueKeys": ["Share of Respondents (%)"],
        "title": "Trends in Tree Preferences",
    },
    {
        "chartId": "line-2",
        "type": "with-area",
        "categoryKey": ["Response"],
        "valueKeys": ["Share of Respondents (%)"],
        "title": "Trends in Tree Preferences",
    },
    {
        "chartId": "scatter-0",
        "type": "basic",
        "categoryKey": ["Response"],
        "valueKeys": ["Share of Respondents (%)"],
        "title": "Respondent Share by Response Type",
    },
    {
        "chartId": "scatter-1",
        "type": "with-size",
        "categoryKey": ["Response"],
        "valueKeys": ["Share of Respondents (%)"],
        "title": "Respondent Share by Response Type",
    },
    {
        "chartId": "area-0",
        "type": "basic",
        "categoryKey": ["Response"],
        "valueKeys": ["Share of Respondents (%)"],
        "title": "Proportion of Tree Choices",
    }
]
\end{lstlisting}

\subsection{Visual Perception}
In this section, we present the generated specifications from visualization interpretation and real-world element understanding. Additionally, the image information is provided in the format: \{"type": "image\_url", "image\_url": \{\}\}.  

\begin{coloredquotation}
    \textbf{Prompt template for visualization specification:}\\
The user will give you a visualization of the data in SVG form \{\textit{SVG}\} and the corresponding visualization in PNG form. Please combine these two outputs with the specification in JSON format:
\begin{lstlisting}[language=TypeScript, label={lst:visualization-class}]
class VisDescription {
/** Chart type (e.g., bar, line, point, area) */
  chartType: string;
  /** Spatial layout and coordinate axes */
  spatialSubstrate: {
    /** Axis definitions mapping data fields */
    axis: { x: string; y: string };
    /** Chart layout variant */
    chartVariants: string;
  }
  /** Visual elements in the chart */
  graphicalElements: {
    mark: {
      /** Mark type (e.g., rect, line, point, arc) */
      type: string;
      role: "dataMarker" | "annotation"; 
      /** Graphical properties and encoding methods */
      graphicalProperties: {
        [key: string]: string;
      }
    }[]
  }
  /** Main insight derived from the visualization */
  visualInsight: string;
}
\end{lstlisting}
\end{coloredquotation}

An example of bar chart specification:
\begin{lstlisting}[language=json, label={lst:visualization-class}]
{
    "visDescription": {
        "chartType": "bar",
        "spatialSubstrate": {
            "axis": { "x": "Continent", "y": "Value" },
            "chartVariants": "stacked"
        },
        "graphicalElements": {
            "mark": [
                {
                    "type": "bar",
                    "role": "dataMarker",
                    "graphicalProperties": {
                        "height": "The height of each bar represents the magnitude of tree cover change for each continent. Bars extend both upward and downward from the x-axis, showing the gross gain and gross loss respectively. Taller bars indicate greater amounts of change.",
                        "color": "Gross gain is represented by light brown (beige) bars, while gross loss is shown in light blue bars. Both colors distinguish the two components of tree cover change in a stacked bar layout."
                    }
                }
            ]
        },
        "visualInsight": "The visualization shows the gross gain and loss of tree cover across various continents. Global has the largest total with both high gross gain and loss. Other continents vary, with differing patterns in their gains and losses."
    }
}
      
\end{lstlisting}

Regarding the description of elements in the real-world image, we also provide entity object information extracted from the narrative intent to assist VLMs in achieving a more accurate understanding of semantic information.
\begin{coloredquotation}
    \textbf{Prompt template for real-world element specification:}\\
The user will provide you with two images: the original image and the masked image of the object in the image outlined with a blue bounding box. 
The user will also provide background information about the image, which includes a narration describing the related event and extracted semantic objects to assist in generating semantic content.
Please combine these two images to output a JSON data format description of the masked object:
\begin{lstlisting}[language=TypeScript, label={lst:visualization-class}]
/** Grain level description: element grouping and geometric type */
class grainLevel {
  /** Single element or grouped elements */
  type: 'singleElement' | 'groupedElements'
  /** Geometric primitive(s): point, line, or plane */
  geometricPrimitive: string | string[]
}

/** Element description within a single element */
class elementDescription {
  /** Spatial layout description of the element */
  layout: string
  /** Geometric shape of the element (e.g., circle, rectangle) */
  shape: string
  /** Semantic role or meaning of the element */
  semantic: string
}

/** Element level description, grouped by geometric primitives */
class ElementLevel {
  /** Plane-level elements (each described by layout, shape, and semantic role) */
  plane: ElementDescription[]
}

class imageDescription {
  /** Grain level: grouping and geometry type */
  grainLevel: GrainLevel
  /** Element level: specific element descriptions */
  elementLevel: ElementLevel
}

\end{lstlisting}
\end{coloredquotation}

An example of the single element specification:
\begin{lstlisting}[language=json, label={lst:visualization-class}]
{
    "imageDescription": {
        "grainLevel": {
            "type": "singleElement",
            "shapeType": "line"
        },
        "elementLevel": {
            "line": {
                "layoutDescription": "A horizontal structure spans across a river or small body of water between trees.",
                "shape": "flattening",
                "semantic": "bridge"
            }
        }
    }
}
\end{lstlisting}

An example of grouped elements specification:
\begin{lstlisting}[language=json, label={lst:visualization-class}]
{
    "imageDescription": {
        "grainLevel": {
            "type": "groupedElements",
            "shapeTypes": [
                "plane"
            ],
            "distributionLayout": "linear"
        },
        "elementLevel": {
            "plane": [
                {
                    "layoutDescription": "The object extends vertically along the center left of the image.",
                    "shape": "rectangle",
                    "semantic": "Real Christmas tree"
                },
                {
                    "layoutDescription": "The object extends vertically along the center right of the image.",
                    "shape": "rectangle",
                    "semantic": "Artificial Christmas tree"
                }
            ]
        }
    }
}
\end{lstlisting}

\subsection{Reasoning and Mapping}
In this section, we present the design and generation of the mapping, along with the associated reasoning process. This includes adjustments to data visualization, as well as the invocation of tools and configuration of parameters during the implementation stage. 

The input of design mapping generation consists of four components:
\begin{itemize}
  \item \textit{Real-world scene image:} A photograph where specific elements are segmented and outlined with blue contours.

  \item \textit{\texttt{imageDescription} (JSON file):} A structured file that describes each segmented element in the form of specification defined before.

  \item \textit{\texttt{visDescription} (JSON file):} A specification of the data visualization as mentioned before.

  \item \textit{\texttt{visSVG} (SVG file):} A vector-based representation of the visualization, which contains all visual elements with unique class names.
\end{itemize}

\begin{coloredquotation}
    \textbf{Prompt template for design mapping:}\\
You are a data analyst and designer specializing in integrating data visualizations into real-world scene images based on narrative intent.
Your task is to analyze the visual features and semantic structures of these inputs and generate creative design proposals that seamlessly integrate the real-world scene with the data visualization. 

Based on prior design experiences, you should refer to the following design patterns to guide your proposal.
Both semantic coherence and visual alignment are important. While achieving both is ideal, satisfying one dimension can still produce effective results.

1. Spatial Organization.\\ A single element in the real-world scene can be mapped to a data marker or a set of data markers sharing the same data attributes, the entire canvas, or coordinate axes. When \texttt{type} is \texttt{singleElement} under \texttt{grainLevel} in \texttt{imageDescription}.
Grouped elements can be mapped to data markers but require a data-binding relationship. When \texttt{type} is \texttt{groupedElements} under \texttt{grainLevel} in \texttt{imageDescription}.

2. Shape Similarity.\\ It involves two types: similar in shape types and similar in shape features. For shape types, the shapes of real-world elements approximate the mark types in data visualizations, such as points to points, lines to lines, and circles to circles. Refer to the \texttt{shapeType} under \texttt{grainLevel} in \texttt{imageDescription} and the \texttt{chartType} or \texttt{type} under \texttt{mark} in \texttt{visDescription}. For shape features, the visual shape features of real-world elements can correspond to the mark \texttt{type} or \texttt{chartType} in the visualization or point to insights from the overall visual representation \texttt{visualInsight} of the data visualization.

3. Layout Consistency\\ We consider relative positions and the distribution here to meet the layout alignment. The relative position of individual elements within a real-world scene can correspond to the spatial layout of a visualization, like serving as the coordinate origin. Consider the \texttt{elementLevel} under \texttt{layoutDescription} in the \texttt{imageDescription} and the \texttt{spatialSubstrate} in the \texttt{visDescription}.
The distribution of grouped elements within a real-world scene corresponds to the overall visualization placement. This should be considered regarding the \texttt{distributionLayout} under \texttt{grainLevel} in \texttt{imageDescription} and the \texttt{spatialSubstrate} or \texttt{visualInsight} in \texttt{visDescription}.

4. Semantic Binding\\
The semantics of real-world entities can directly correspond to the meaning of the data or metaphorically represent data categories. Additionally, elements conveying narrative context can also be mapped accordingly. This rule can be considered by referring to the \texttt{semantic} in \texttt{imageDescription} and metadata information in \texttt{visualInsight}.

If no design mapping exists, return None. If a design mapping exists, please provide your design proposal in the following JSON structure:
\begin{lstlisting}[language=TypeScript, label={lst:visualization-class}]
/** Overview of the entire design plan */
class designPlan {
  /** General overview description of the design plan */
  overview: string
  /** List of mapping plans connecting real-world elements to visualization elements */
  mappingPlan: MappingPlan[]
}

/** Description of a single mapping between real-world and visualization elements */
class mappingPlan {
  /** Type of mapping */
  mappingType: 'one-to-one' | 'one-to-many' | 'many-to-many'
  /** Names or IDs of real-world elements involved */
  realWorldElements: string[]
  /** Names or IDs of visualization elements involved */
  visElements: string[]
  /** Optional: semantic alignment if available */
  semanticAlignment?: SemanticAlignment
  /** Optional: visual alignment if available */
  visualAlignment?: VisualAlignment
}

/** Description of semantic alignment between data visualization and real-world elements */
class semanticAlignment {
  /** Semantic meaning in the data visualization (e.g., category, metric, label, auxiliary fuction) */
  visSemantic: string
  /** Semantic meaning in the real-world element (e.g., object role, contextual meaning) */
  realWorldSemantic: string
  /** Explanation of the semantic relationship and its intended effect */
  description: string
}


/** Description of visual alignment: shape and layout matching */
class visualAlignment {
  /** Optional: shape alignment if available */
  shapeAlignment?: ShapeAlignment
  /** Optional: layout alignment if available */
  layoutAlignment?: LayoutAlignment
}

/** Shape alignment: visual shape mapping description */
class shapeAlignment {
  /** Shape or visual feature of the real-world element */
  realWorldShape: string
  /** Corresponding visualization element shape */
  visShape: string
  /** Explanation of shape alignment logic and its visual effect */
  description: string
}

/** Layout alignment: spatial arrangement mapping description */
class layoutAlignment {
  /** Layout or positioning of real-world elements */
  realWorldLayout: string
  /** Layout or positioning in the visualization */
  visLayout: string
  /** Alignment type: e.g., center, bottom-left, bottom-right, top-left, top-right */
  alignmentType: 'center' | 'bottom-left' | 'bottom-right' | 'top-left' | 'top-right'
  /** Explanation of layout alignment and its spatial effect */
  description: string
}
\end{lstlisting}
\end{coloredquotation}

An example of mapping design:
\begin{lstlisting}[language=json, label={lst:visualization-class}]
{
  "designPlan": {
    "overview": "Integrate the Ferris wheel in the real-world scene with the donut chart visual, aligning the circular shapes for thematic cohesion and enhancing storytelling through visual symbolism.",
    "mappingPlan": [
      {
        "realWorldElements": ["#ferris-wheel"],
        "mappingType": "one-to-one",
        "visElements": ["#donut-chart"],
        "semanticAlignment": {
          "dataSemantic": "Age groups in merchandise sales",
          "realWorldSemantic": "Ferris wheel symbolizing cycles and diversity",
          "description": "The Ferris wheel metaphorically represents the cyclical and inclusive nature of age diversity in merchandise sales."
        },
        "visualAlignment": {
          "shapeAlignment": {
            "realWorldShape": "Circle",
            "visShape": "Donut",
            "description": "Both the Ferris wheel and the donut chart share a circular shape."
          },
          "layoutAlignment": {
            "realWorldLayout": "Upper-left quadrant of the scene",
            "visLayout": "Center of the visualization canvas",
            "alignmentType": "center",
            "description": "The prominent position of the Ferris wheel in the upper-left quadrant aligns with the central placement of the donut chart."
          }
        }
      }
    ]
  }
}
\end{lstlisting}

For all design mappings, we submit a request and recommendation regarding the necessity of data visualization adjustments, which include both data-level and view-level modifications. If the model determines that appropriate visualization adjustments can achieve improved mapping without altering the correctness of the data fact, it can utilize relevant parameters and return a corresponding list of functions.

\begin{coloredquotation}
    \textbf{Prompt template for visualization adjustment and tool execution:}\\
You may propose reasonable modifications to the visualization view to support the integration, but these changes must respect visualization principles and maintain data narrative consistency. Modifications can occur both at the data level and the view level.

At the data level, you are allowed to improve entity-to-data mapping by filtering or pruning the dataset using the function \texttt{filterData(dataset, filterCondition)}, where \texttt{dataset} is the input data collection and \texttt{filterCondition} defines the rule for selecting relevant entities. You can also sort the dataset to highlight key insights by applying \texttt{sortData(dataset, sortKey, sortOrder)}, where \texttt{sortKey} specifies the attribute for sorting and \texttt{sortOrder} determines whether the sorting is ascending, descending or other orders. To better structure the information, you may categorize the data using \texttt{categorizeData(dataset, categoryKey)}, grouping entities based on a shared attribute.

At the view level, adjustments should aim to better align visual elements with real-world scene representations while preserving clarity and meaning. You may resize elements by applying \texttt{editSvgSize(SvgElement, targetHeight, targetWidth)}, shift their positions using \texttt{editSvgPosition(SvgElement, targetX, targetY)}, or adjust their orientation through \texttt{editSvgRotation(SvgElement, targetAngle)}. Before that, you should select and align the anchor point to modify these operations using \texttt{alignToElement(source, target, alignmentType)}.

Finally, you should return a sequence of the applied operations in the form of function calls with their arguments.
\end{coloredquotation}
An example of function calls is as follows:
\begin{lstlisting}[language=json, label={lst:visualization-class}]
[
  "alignToElement('radarChart', 'cityCenter', 'center')",
  "editSvgPosition('radarChart', cityCenter.center.x, cityCenter.center.y)",
  "editSvgSize('radarChart', cityCenter.boundingBox.xmax - cityCenter.boundingBox.xmin, cityCenter.boundingBox.ymax - cityCenter.boundingBox.ymin)"
]
\end{lstlisting}

All elements specified in the mapping plan are represented using class names for element access. We employ the following approach for parameter storage and access for the basic parameters of point, line, and plane elements in real-world scenes.
\begin{lstlisting}[language=TypeScript, label={lst:visualization-class}]
/** Point element: describes key attributes for alignment */
class Point {
  /** x coordinate of the point */
  x: number
  /** y coordinate of the point */
  y: number
  /** Size of the point */
  size?: number
  /** Color of the point */
  color?: string
  /** Semantic label */
  label?: string
  /** Bounding box of the point */
  boundingBox?: { xmin: number, ymin: number, xmax: number, ymax: number }
}

/** Line element: describes key attributes for alignment */
class Line {
  /** Start x coordinate */
  x1: number
  /** Start y coordinate */
  y1: number
  /** End x coordinate */
  x2: number
  /** End y coordinate */
  y2: number
  /** Width of the line */
  width?: number
  /** Color of the line */
  color?: string
  /** Semantic label */
  label?: string
  /** Center point of the line (optional, pre-calculated) */
  center?: { sx: number, y: number}
  /** Length of the line */
  length?: number
  /** Angle of the line to the horizontal */
  angle?: number
  /** Bounding box of the line  */
  boundingBox?: { xmin: number, ymin: number, xmax: number, ymax: number }
}

/** Plane element: describes key attributes for alignment */
class Plane {
  /** List of boundary points defining the plane */
  boundaryPoints: { x: number, y: number}[]
  /** Semantic label */
  label?: string
  /** Center point of the plane */
  center?: {x: number, y: number}
  /** Shape type: e.g., rectangle, polygon, circle */
  shapeType?: string
  /** Aspect ratio (width / height) of the plane */
  aspectRatio?: number
  /** Bounding box of the plane */
  boundingBox?: { xmin: number, ymin: number, xmax: number, ymax: number }
}
\end{lstlisting}

The relevant tools and parameters are listed in Table.~\ref{tab: tool execution}.

\begin{table}[h]
\centering
\vspace{-0.2cm}
\caption{Tools for manipulating SVG elements in data visualization.}
\vspace{-0.2cm}
\label{tab: tool execution}
\begin{tabular}{l p{5.8cm}}
\hline
\textbf{Tool} & \textbf{Parameters} \\
\hline
getSvgElement & (SvgPath, className) \\
editSvgSize & (SvgElement, targetHeight, targetWidth) \\
editSvgPosition & (SvgElement, targetX, targetY) \\
editSvgRotation & (SvgElement, targetAngle) \\
alignToElement & (source, target, alignmentType) \\
\hline
\end{tabular}
\vspace{-0.4cm}
\end{table}

\subsection{Design Evaluation}
This section presents our method for evaluating and providing suggestions for a design alternative, including assessments of data accuracy and visual clarity. Particular attention is given to determining whether instances of data conflict require handling through inpainting operations.

\begin{coloredquotation}
    \textbf{Prompt template for design evaluation:}\\
We are evaluating the effectiveness of a visualization that combines data graphics with real-world imagery. A structured data table will be provided as the ground truth. You are asked to assess the visualization based on both the visual content and the provided data table.

For data accuracy, you should evaluate whether the integration of visual elements (charts, marks, overlays) with the image accurately conveys the underlying data, and whether data values, trends, or relationships are clearly and correctly represented. Additionally, you must check for any conflicts between the visualization and the data table. If a conflict is detected, determine whether inpainting is necessary. If inpainting is needed, you should provide the coordinates of the point where correction should occur (point\_coords), and assess whether there are existing elements that can be reused (reusable\_element). If a reusable element is available, the method remove\_anything.py should be applied. If no reusable element is available, the method fill\_anything.py should be used instead, and a semantic text prompt (text\_prompt) must be provided to guide the inpainting process.

For readability and clarity, you should assess whether the visualization is easy to understand at a glance, whether the incorporation of the image enhances or hinders the viewer's interpretation of the data, and whether visual elements such as labels, highlights, colors, and scales are clear and distinguishable.

Your evaluation should include a score for each category on a scale of 1 (very poor) to 5 (excellent), accompanied by a brief explanation supporting your assessment. The data table should be used to substantiate your evaluation of accuracy.

Please format your evaluation results in the following JSON structure:
\begin{lstlisting}[language=Typescript, label={lst:visualization-class}]
/** Evaluation result for design effectiveness */
class evaluationResult {
  /** Evaluation of data representation accuracy */
  data_accuracy: DataAccuracy
  /** Evaluation of visualization readability and clarity */
  readability: Readability
}

/** Details about data accuracy evaluation */
class dataAccuracy {
  /** Score from 1 (very poor) to 5 (excellent) */
  score: number
  /** Brief explanation supporting the score */
  explanation: string
  /** Whether a conflict between visualization and ground-truth data is detected */
  conflict_detected: boolean
  /** Inpainting operation details if a conflict exists */
  inpaint_operation?: InpaintOperation
}

/** Inpainting operation specification */
class inpaintOperation {
  /** Whether inpainting is required */
  need_inpaint: boolean
  /** Coordinates indicating correction points */
  point_coords: {
    /** X coordinate of the correction point */
    x: number
    /** Y coordinate of the correction point */
    y: number
  }[]
  /** Whether an existing visual element can be reused */
  reusable_element: boolean
  /** Selected method for inpainting: reuse or semantic fill */
  method: 'remove_anything.py' | 'fill_anything.py'
  /** Textual prompt describing the semantic content if using "fill_anything.py" */
  text_prompt?: string
}

/** Details about readability evaluation */
class readability {
  /** Score from 1 (very poor) to 5 (excellent) */
  score: number
  /** Brief explanation supporting the score */
  explanation: string
}


\end{lstlisting}
\end{coloredquotation}

An example of design evaluation:
\begin{lstlisting}[language=json, label={lst:visualization-class}]
{
  "data_accuracy": {
    "score": 3,
    "explanation": "Data points incorrectly placed.",
    "conflict_detected": true,
    "inpaint_operation": {
      "need_inpaint": true,
      "point_coords": [
        { "x": 320, "y": 210 },
        { "x": 450, "y": 310 }
      ],
      "reusable_element": true,
      "method": "fill_anything.py",
      "text_prompt": "the blue sky."
    }
  },
  "readability": {
    "score": 3,
    "explanation": "Visualization is mostly clear, slight label overlaps."
  }
}

\end{lstlisting}

The command templates for executing removal or filling operations via inpainting are as follows:
\begin{lstlisting}[language=json, label={lst:visualization-class}]
python remove_anything.py \
    --input_img {input_img_path} \
    --coords_type {coords_type} \
    --point_coords {point_coords} \
    --point_labels {point_labels} \
    --dilate_kernel_size {dilate_kernel_size} \
    --output_dir {output_dir} \
    --sam_model_type {sam_model_type} \
    --sam_ckpt {sam_ckpt_path} \
    --lama_config {lama_config_path} \
    --lama_ckpt {lama_ckpt_path}

python fill_anything.py \
    --input_img {input_img_path} \
    --coords_type {coords_type} \
    --point_coords {point_coords} \
    --point_labels {point_labels} \
    --text_prompt "{text_prompt}" \
    --dilate_kernel_size {dilate_kernel_size} \
    --output_dir {output_dir} \
    --sam_model_type {sam_model_type} \
    --sam_ckpt {sam_ckpt_path}
\end{lstlisting}

\subsection{Animation Generation}
This section demonstrates the prompt for generating animations for SVG-based design alternatives. We will use the action descriptions obtained from feature extraction in narrative intents as references to generate Anime.js~\cite{animejs} code for animation production. The prompt design refers to the related work by Shen et al.~\cite{shen2024dataplayer, shen2024dataplaywright} to guide the model in understanding the relationships between data visualization and animation types.

\begin{coloredquotation}
    \textbf{Prompt template for animation generation:}\\
You are an expert in generating animations for SVG elements using anime.js. Based on the natural language description of the animation \{\textit{actions}\} and the provided SVG file \{\textit{SVG}\}, first identify the target elements that require animation. Then, according to the description and the characteristics of data visualization, generate the corresponding anime.js animation code.

You may use the following animation guidelines as a reference:\\
- Axes-fade-in: Apply changes in opacity and strokeWidth to elements with the class '.axis' (opacity: [0,1], strokeWidth: [0,2], duration: 800) — used for rendering coordinate axes.\\
- Bar-grow-in: Animate height and translateY with elasticity (height: ['0\%', '100\%'], translateY: [50,0], elasticity: 300, stagger: 100) — used for animating bar chart columns.\\
- Line-wipe-in: Animate strokeDashoffset (strokeDashoffset: [anime.setDashoffset, 0], duration: 1500) — used for line chart paths.\\
- Pie-wheel-in: Apply rotation and scaling (rotate: ['-90deg', '0deg'], scale: [0,1], easing: 'spring(1, 80, 10, 0)') — used for animating pie chart sectors.\\
- Float-in: Animate translateY/translateX and opacity (translateY: ['20px', '0'], opacity: [0,1], direction: 'top', delay: 200) — used for floating tooltips or annotations.\\
- Change-color: Change the fill color (fill: ['\#ccc', '\#f00'], duration: 500) for elements with the selector \eg '.bar[data-value>50]'.\\

Please return the animation in the following JSON structure:
\begin{lstlisting}[language=Typescript, label={lst:visualization-class}]
/** Configuration for anime.js animation */
class animeJSConfig {
  /** CSS selector, DOM element, or array of elements to animate */
  targets: string | HTMLElement | HTMLElement[]
  /** Type of animation: entrance, emphasis, or exit */
  animation_type: 'entrance' | 'emphasis'
  /** Animation properties depending on the animation type */
  properties: {
    /** Key-value pairs for property animation, e.g., opacity: [0, 1] */
    [propertyName: string]: [string | number, string | number]
    /** Direction of animation movement */
    direction?: 'top' | 'bottom' | 'left' | 'right'
  }
  /** Timing control for the animation */
  timing: {
    /** Total duration of the animation in milliseconds */
    duration: number
    /** Delay before the animation starts in milliseconds */
    delay: number
  }
}
\end{lstlisting}

\end{coloredquotation}

An example of generated animation for bar chart:
\begin{lstlisting}[language=json, label={lst:visualization-class}]
{
  targets: '.bar',
  animation_type: 'entrance',
  properties: {
    scaleY: [0, 1],
    opacity: [0, 1],
    direction: 'bottom'
  },
  timing: {
    duration: 800,
    delay: 100
  }
}
\end{lstlisting}

\section{Evaluation Details}
We provide supplementary materials to support our evaluation of SceneLoom, including: (1) a small-scale assessment of LLM usage cost during the generation process, (2) a detailed explanation of the user study procedure, and (3) the complete questionnaires and response results for the user study. In addition, design outcomes produced by participants are presented in a packaged format within the \textit{Examples} folder.

\subsection{LLM Usage Cost}
To assess the efficiency and resource consumption of the generation process, we track two key metrics throughout the workflow:
\textit{Time Elapsed} and \textit{Token Usage}. We measure the total time required for LLM to generate the output using Python’s time module. Timestamps are recorded before and after the model call, and the difference yields the elapsed time in seconds. Token usage is estimated using OpenAI’s tiktoken library~\cite{tiktoken} to encode the input tokens and the model's response. The total token count is computed by summing the number of tokens in each of these segments.

We further evaluated a set of five representative cases across a three-stage workflow: data preparation, which involves generating the initial visualizations, extracting key features, and constructing structured specifications; reasoning and mapping, where mapping strategies are generated and relevant tools are invoked and adjusted accordingly; and evaluation, which assesses the accuracy of data representations, visual clarity, and attention guidance.
In each case, we also recorded the number of generated design elements or alternatives, as this directly affects both computation time and potential economic cost.

\begin{figure}[t]
% \vspace{-0.3cm}
  \centering 
  \includegraphics[width=\columnwidth]{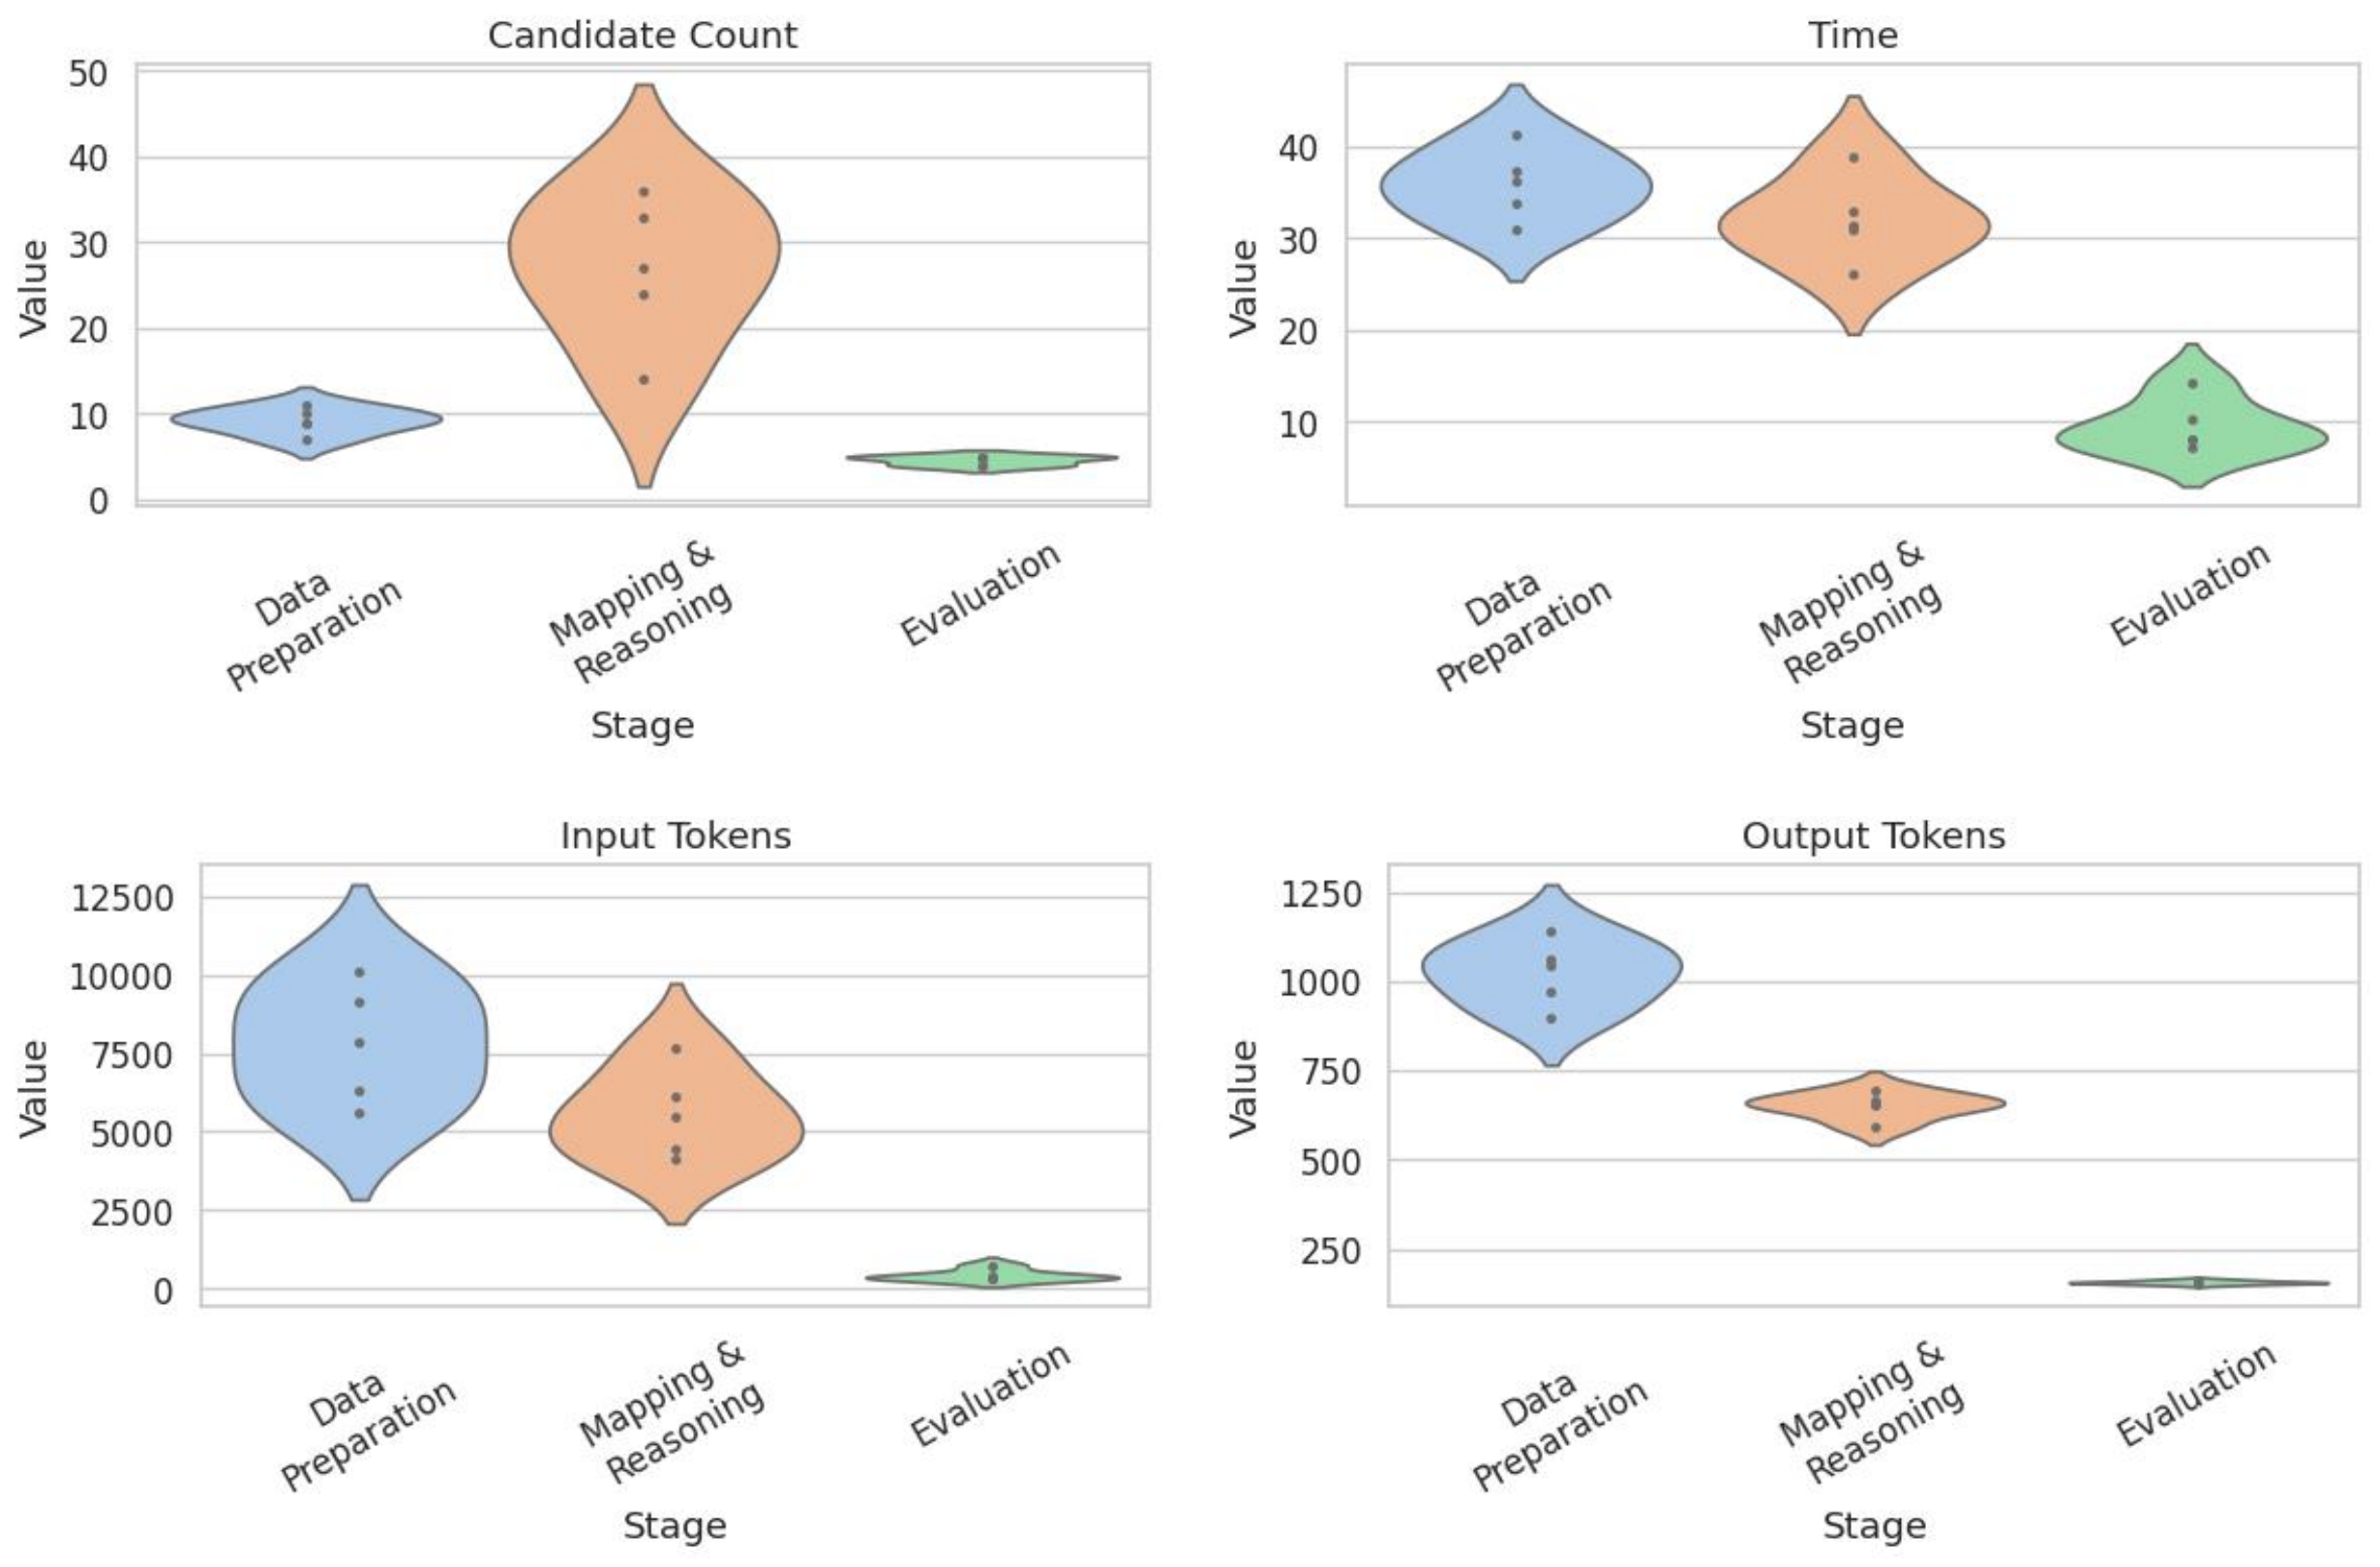}
  \caption{Distribution of four computational metrics. }
  \label{fig: llm cost}
  \vspace{-0.5cm}
\end{figure}

To understand the end-to-end computational cost, we aggregate metric values across the three workflow stages, as illustrated in Fig.~\ref{fig: llm cost}. On average, each case takes 77.6 seconds, consumes 13,803 input tokens, and produces 1,832 output tokens. The largest variance is observed in input token usage, indicating differences in input length and reasoning complexity.

Across each stage, we observe a consistent trend in time and token usage. Mapping \& Reasoning is the most resource-intensive stage, with the highest candidate count ($M$=26.8), while Evaluation is the most lightweight, both in execution time ($M$=9.2) and token consumption ($M$=433.0; $M$=157.3). These results highlight the middle stage as the key computational bottleneck and suggest potential for optimization through candidate pruning or reasoning efficiency.

\subsection{User Study Protocol}
\textbf{Participants:} 10 individuals were invited to participate in the evaluation study, with an even distribution of 4 male and 6 female participants.

\textbf{Procedure:}

1. The purpose and process of our user study will be explained to all participants. We will also present five representative examples from our collected corpus to more vividly illustrate the research content and experimental objectives to the participants. (duration: 5min)

2. Participants are first required to complete a \textit{\textbf{self-report}} evaluating their level of expertise or experience in fields related to data visualization, visual design, and video editing. We employ a 5-point Likert scale, where participants rate their expertise, with 1 indicating no experience and 5 indicating expert-level proficiency. (duration: 5min)

3. We present ten groups of datasets covering different themes and formats. After a brief introduction, participants independently select two datasets as tasks in the subsequent experiment. We guide participants to gain a deeper understanding of each dataset and encourage them to freely articulate their ideas on how to approach the design, either through verbal descriptions or by sketching. (duration: 10min)

4. We first introduce the basic workflow and interaction features of our system through an example. Participants then use SceneLoom to work on the two assigned tasks. During the creation process, we require them to think aloud while we observe their design activities. Finally, we save the participants' final design outcomes. (duration: 20min)

5. At the end of the study, we ask participants to complete a \textbf{\textit{subjective questionnaire}} and a semi-structured interview regarding their usage experience and satisfaction with SceneLoom. The questions involved in the questionnaire are shown in Table.~\ref{tab: self-report}. (duration: 10min)

\begin{table}[htbp]
\centering
\small
\caption{Domains and associated questions in user evaluation}
\begin{tabular}{ll}
\hline
\textbf{Domain} & \textbf{Question} \\
\hline
\multirow{2}{*}{Usability} 
& Q1: Satisfied with interface design and interactions. \\
& Q2: Easy to understand and use. \\
\hline
\multirow{2}{*}{Effectiveness} 
& Q3: Enables exploratory and creative design process. \\
& Q4: Satisfied with the design outcomes. \\
\hline
\multirow{2}{*}{Recommendations} 
& Q5: Engaging and enjoyable design experience. \\
& Q6: Likely to recommend SceneLoom to others. \\
\hline
\end{tabular}
\label{tab: self-report}
\end{table}

\subsection{Questionnaires and Results}
The self-report scores of the 10 participants (P1-P10) regarding their level of expertise on data visualization, visual design and video editing are presented in Table.~\ref{tab: self-repot result}. Among them, P1 and P2 are data analysts, P3 is a journalist, P4 and P8 are HCI researchers, P5 and P7 are designers, and P6 and P9 are VIS researchers.
\begin{table}[htbp]
\centering
\small
\caption{Participant self-reports on experience levels}
\begin{tabular}{lcccccccccc@{\hskip 3pt}c}
\hline
 & P1 & P2 & P3 & P4 & P5 & P6 & P7 & P8 & P9 & P10 & $M\pm Std $ \\
\hline
Vis & 4 & 3 & 3 & 4 & 3 & 5 & 5 & 4 & 5 & 2 & $3.8\pm1.03$ \\
Design & 2 & 3 & 3 & 3 & 5 & 4 & 4 & 4 & 3 & 3 & $3.4\pm0.84$ \\
Video & 4 & 2 & 5 & 2 & 3 & 2 & 4 & 5 & 4 & 3 & $3.4\pm1.17$ \\
\hline
\end{tabular}
\label{tab: self-repot result}
\end{table}

User feedback on their experience with SceneLoom and their satisfaction with the design outcomes is presented in Table.~\ref{tab: user feedback}. The results in this table are consistent with the user rating results for the subjective questions as presented in the main text.

\begin{table}[htbp]
\centering
\small
\caption{Participant ratings on user experience of SceneLoom}
\begin{tabular}{lccccccccccc}
\hline
 & P1 & P2 & P3 & P4 & P5 & P6 & P7 & P8 & P9 & P10 & $M \pm Std$ \\
\hline
Q1 & 4 & 4 & 5 & 4 & 5 & 5 & 4 & 4 & 5 & 4 & $4.4\pm0.52$ \\
Q2 & 5 & 5 & 5 & 4 & 4 & 5 & 4 & 3 & 5 & 4 & $4.4\pm0.70$ \\
Q3 & 4 & 4 & 5 & 5 & 5 & 5 & 4 & 5 & 5 & 5 & $4.7\pm0.48$ \\
Q4 & 4 & 5 & 4 & 4 & 4 & 5 & 4 & 5 & 2 & 3 & $4.0\pm0.94$ \\
Q5 & 4 & 4 & 5 & 5 & 5 & 5 & 5 & 5 & 4 & 3 & $4.5\pm0.71$ \\
Q6 & 4 & 5 & 4 & 5 & 5 & 5 & 4 & 5 & 5 & 4 & $4.6\pm0.52$ \\
\hline
\end{tabular}
\label{tab: user feedback}
\end{table}
